# Supplementary material for: Probabilistic Shaping for the AWGN Channel
Source: arXiv:2302.08388 source file (2023-02-16)
Supplement: Supplementary file 2 [file AppendixTemplate.tex]

% Appendix Template

\chapter{Appendix Title Here} % Main appendix title

\label{AppendixX} % Change X to a consecutive letter; for referencing this appendix elsewhere, use \ref{AppendixX}

Write your Appendix content here.
